# Supplementary material for: Magnon Thermal Hall Effect Induced By Symmetric Exchange Interaction
Source: arXiv:2501.02250 source file (2025-12-19)
Supplement: Supplementary file 1 [file SupplementalMaterial.pdf]

# Supplemental material for “Magnon Thermal Hall Effect Induced By Symmetric Exchange Interaction”

Jikun Zhou,<sup>1</sup> Yang Gao,<sup>1,2</sup> and Qian Niu<sup>1,2</sup>

<sup>1</sup>*CAS Key Laboratory of Strongly-Coupled Quantum Matter Physics and Department of Physics, University of Science and Technology of China, Hefei, Anhui 230026, China*

<sup>2</sup>*Hefei National Laboratory, University of Science and Technology of China, Hefei 230088, China*

(Dated: April 27, 2025)

## I. MATRIX FORM OF GENERALIZED HEISENBERG HAMILTONIAN

In this section, we will derive the matrix element of local spin Hamiltonian, i.e., Eq.(3) and Eq.(4) of manuscript in detail. Consider a generalized Heisenberg Hamiltonian

$$H = \frac{1}{2} \sum_{n,m} \sum_{i,j} \sum_{ab} \mathbf{S}_{n,i}^a J_{ni,mj}^{ab} \mathbf{S}_{m,j}^b, \quad (\text{S1})$$

and we only care about bilinear terms so that interaction tensor  $J_{ni,mj}$  will have the form

$$J_{ni,mj} = \begin{bmatrix} J_{ni,mj}^{xx} & J_{ni,mj}^{xy} & 0 \\ J_{ni,mj}^{yx} & J_{ni,mj}^{yy} & 0 \\ 0 & 0 & J_{ni,mj}^z \end{bmatrix}. \quad (\text{S2})$$

Thus we can expand Eq. (S1) and use definition of ladder operators  $S_{n,i}^{\pm} = S_{n,i}^x \pm iS_{n,i}^y$ ,

$$\begin{aligned} H &= \frac{1}{2} \sum_{n,m} \sum_{i,j} (S_{n,i}^x, S_{n,i}^y, S_{n,i}^z) \begin{bmatrix} J_{ni,mj}^{xx} & J_{ni,mj}^{xy} & 0 \\ J_{ni,mj}^{yx} & J_{ni,mj}^{yy} & 0 \\ 0 & 0 & J_{ni,mj}^z \end{bmatrix} \begin{pmatrix} S_{m,j}^x \\ S_{m,j}^y \\ S_{m,j}^z \end{pmatrix} \\ &= \frac{1}{2} \sum_{n,m} \sum_{i,j} J_{ni,mj}^{xx} S_{n,i}^x S_{m,j}^x + J_{ni,mj}^{yy} S_{n,i}^y S_{m,j}^y + J_{ni,mj}^{xy} S_{n,i}^x S_{m,j}^y + J_{ni,mj}^{yx} S_{n,i}^y S_{m,j}^x + J_{ni,mj}^{zz} S_{n,i}^z S_{m,j}^z \\ &= \frac{1}{2} \sum_{n,m} \sum_{i,j} \left\{ J_{ni,mj}^{xx} \frac{S_{n,i}^+ + S_{n,i}^-}{2} \frac{S_{m,j}^+ + S_{m,j}^-}{2} + J_{ni,mj}^{yy} \frac{S_{n,i}^+ - S_{n,i}^-}{2i} \frac{S_{m,j}^+ - S_{m,j}^-}{2i} \right. \\ &\quad \left. + J_{ni,mj}^{xy} \frac{S_{n,i}^+ + S_{n,i}^-}{2} \frac{S_{m,j}^+ - S_{m,j}^-}{2i} + J_{ni,mj}^{yx} \frac{S_{n,i}^+ - S_{n,i}^-}{2i} \frac{S_{m,j}^+ + S_{m,j}^-}{2} \right\} + J_{ni,mj}^{zz} S_{n,i}^z S_{m,j}^z \\ &= \frac{1}{2} \sum_{n,m} \sum_{i,j} \frac{1}{4} \left\{ [J_{ni,mj}^{xx} - J_{ni,mj}^{yy} - i(J_{ni,mj}^{xy} + J_{ni,mj}^{yx})] S_{n,i}^+ S_{m,j}^+ + [J_{ni,mj}^{xx} + J_{ni,mj}^{yy} + i(J_{ni,mj}^{xy} - J_{ni,mj}^{yx})] S_{n,i}^+ S_{m,j}^- \right. \\ &\quad \left. + [J_{ni,mj}^{xx} + J_{ni,mj}^{yy} - i(J_{ni,mj}^{xy} - J_{ni,mj}^{yx})] S_{n,i}^- S_{m,j}^+ + [J_{ni,mj}^{xx} - J_{ni,mj}^{yy} + i(J_{ni,mj}^{xy} + J_{ni,mj}^{yx})] S_{n,i}^- S_{m,j}^- \right\} \\ &\quad + J_{ni,mj}^{zz} S_{n,i}^z S_{m,j}^z. \end{aligned} \quad (\text{S3})$$

By the means of Holstein-Primakoff transformation [S1]

$$S_{n,i}^+ \approx \sqrt{2S} a_{n,i}, \quad S_{n,i}^- \approx \sqrt{2S} a_{n,i}^\dagger, \quad S_{n,i}^z = S - a_{n,i}^\dagger a_{n,i}, \quad (\text{S4})$$

Hamiltonian can be turned into

$$\begin{aligned}
H = \frac{S}{2} \sum_{n,m} \sum_{i,j} \frac{1}{2} \bigg\{ & [J_{ni,mj}^{xx} - J_{ni,mj}^{yy} - i(J_{ni,mj}^{xy} + J_{ni,mj}^{yx})] a_{n,i} a_{m,j} + [J_{ni,mj}^{xx} + J_{ni,mj}^{yy} + i(J_{ni,mj}^{xy} - J_{ni,mj}^{yx})] a_{n,i} a_{m,j}^\dagger \\
& + [J_{ni,mj}^{xx} + J_{ni,mj}^{yy} - i(J_{ni,mj}^{xy} - J_{ni,mj}^{yx})] a_{n,i}^\dagger a_{m,j} + [J_{ni,mj}^{xx} - J_{ni,mj}^{yy} + i(J_{ni,mj}^{xy} + J_{ni,mj}^{yx})] a_{n,i}^\dagger a_{m,j}^\dagger \bigg\} \\
& - J_{ni,mj}^{zz} (a_{n,i}^\dagger a_{n,i} + a_{m,j}^\dagger a_{m,j}).
\end{aligned} \tag{S5}$$

Through Fourier transform of creation and annihilation operators:  $a_{n,i} = (1/\sqrt{N}) \sum_{\mathbf{k}} e^{i\mathbf{k} \cdot (\mathbf{R}_n + \mathbf{r}_i)} a_{i,\mathbf{k}}$  and  $a_{n,i}^\dagger = (1/\sqrt{N}) \sum_{\mathbf{k}} e^{-i\mathbf{k} \cdot (\mathbf{R}_n + \mathbf{r}_i)} a_{i,\mathbf{k}}^\dagger$ , we get Hamiltonian in momentum space

$$\begin{aligned}
H = \frac{S}{2} \sum_{n,m} \sum_{i,j} \frac{1}{2} \bigg\{ & [J_{ni,mj}^{xx} - J_{ni,mj}^{yy} - i(J_{ni,mj}^{xy} + J_{ni,mj}^{yx})] e^{-i\mathbf{k} \cdot (\mathbf{R}_{mj} - \mathbf{R}_{ni})} a_{i,\mathbf{k}} a_{j,-\mathbf{k}} \\
& + [J_{ni,mj}^{xx} + J_{ni,mj}^{yy} + i(J_{ni,mj}^{xy} - J_{ni,mj}^{yx})] e^{-i\mathbf{k} \cdot (\mathbf{R}_{mj} - \mathbf{R}_{ni})} a_{i,\mathbf{k}} a_{j,\mathbf{k}}^\dagger \\
& + [J_{ni,mj}^{xx} + J_{ni,mj}^{yy} - i(J_{ni,mj}^{xy} - J_{ni,mj}^{yx})] e^{i\mathbf{k} \cdot (\mathbf{R}_{mj} - \mathbf{R}_{ni})} a_{i,\mathbf{k}}^\dagger a_{j,\mathbf{k}} \\
& + [J_{ni,mj}^{xx} - J_{ni,mj}^{yy} + i(J_{ni,mj}^{xy} + J_{ni,mj}^{yx})] e^{i\mathbf{k} \cdot (\mathbf{R}_{mj} - \mathbf{R}_{ni})} a_{i,\mathbf{k}}^\dagger a_{j,-\mathbf{k}}^\dagger \bigg\} - J_{ni,mj}^{zz} (a_{i,\mathbf{k}}^\dagger a_{i,\mathbf{k}} + a_{j,\mathbf{k}}^\dagger a_{j,\mathbf{k}}).
\end{aligned} \tag{S6}$$

Finally, we can turn this Hamiltonian to matrix form by choosing basis  $\psi_{\mathbf{k}} = (a_{1,\mathbf{k}}, \dots, a_{N,\mathbf{k}}, a_{1,-\mathbf{k}}^\dagger, \dots, a_{N,-\mathbf{k}}^\dagger)^T$ ,

$$H = \sum_{\mathbf{k}} \psi_{\mathbf{k}}^\dagger \mathcal{H}_{\mathbf{k}} \psi_{\mathbf{k}} = \sum_{\mathbf{k}} \psi_{\mathbf{k}}^\dagger \frac{S}{2} \begin{bmatrix} \mathbf{A}(\mathbf{k}) & \mathbf{B}(\mathbf{k}) \\ \mathbf{B}^*(-\mathbf{k}) & \mathbf{A}^*(-\mathbf{k}) \end{bmatrix} \psi_{\mathbf{k}}. \tag{S7}$$

And we have shown that, submatrices  $\mathbf{A}(\mathbf{k})$  and  $\mathbf{B}(\mathbf{k})$  are [S2]

$$\begin{aligned}
[\mathbf{A}(\mathbf{k})]_{i,j} &= \sum_{m,n} \frac{1}{2} [J_{ni,mj}^{xx} + J_{ni,mj}^{yy} - i(J_{ni,mj}^{xy} - J_{ni,mj}^{yx})] e^{i\mathbf{k} \cdot (\mathbf{R}_{mj} - \mathbf{R}_{ni})} - \delta_{ij} \sum_{\ell} J_{ni,m\ell}^{iz,\ell z}, \\
[\mathbf{B}(\mathbf{k})]_{i,j} &= \sum_{m,n} \frac{1}{2} [J_{ni,mj}^{xx} - J_{ni,mj}^{yy} + i(J_{ni,mj}^{xy} + J_{ni,mj}^{yx})] e^{i\mathbf{k} \cdot (\mathbf{R}_{mj} - \mathbf{R}_{ni})}.
\end{aligned} \tag{S8}$$

By denoting  $J_{ni,mj}^{xx} + J_{ni,mj}^{yy} \rightarrow J_{ni,mj}^+$ ,  $J_{ni,mj}^{xx} - J_{ni,mj}^{yy} \rightarrow J_{ni,mj}^-$ ,  $J_{ni,mj}^{xy} - J_{ni,mj}^{yx} \rightarrow D_{ni,mj}$ ,  $J_{ni,mj}^{xy} + J_{ni,mj}^{yx} \rightarrow \Gamma_{ni,mj}$ , we finally arrive at Eq.(3) in main text

$$\begin{aligned}
A_{ij}(\mathbf{k}) &= \sum_{m,n} \frac{1}{2} (J_{ni,mj}^+ - iD_{ni,mj}) e^{i\mathbf{k} \cdot (\mathbf{R}_{mj} - \mathbf{R}_{ni})} - \delta_{ij} \sum_{m\ell} J_{ni,m\ell}^{zz}, \\
B_{ij}(\mathbf{k}) &= \sum_{m,n} \frac{1}{2} (J_{ni,mj}^- + i\Gamma_{ni,mj}) e^{i\mathbf{k} \cdot (\mathbf{R}_{mj} - \mathbf{R}_{ni})}.
\end{aligned} \tag{S9}$$

The Hamiltonian in Eq.(S7) is a bosonic Bogoliubov-de Gennes(BdG) Hamiltonian and can be diagonalized by using para-unitary transformation [S3–S7]

$$T_{\mathbf{k}}^\dagger \mathcal{H}_{\mathbf{k}} T_{\mathbf{k}} = \Sigma_z \begin{bmatrix} E_{\mathbf{k}} & \\ & -E_{-\mathbf{k}} \end{bmatrix}, \tag{S10}$$

where  $E_{\mathbf{k}} = \text{diag}(\varepsilon_{1,\mathbf{k}}, \varepsilon_{2,\mathbf{k}}, \dots, \varepsilon_{N,\mathbf{k}})$  and  $\Sigma_z = \sigma_z \otimes \mathbb{I}_N$  with  $\sigma_z$  being the Pauli matrix and  $\mathbb{I}_N$  being the  $N \times N$  unit matrix. The structure of the eigen energy is due to particle-hole symmetry which is a typical symmetry of magnon BdG Hamiltonian [S5–S7]. In order to maintain bosonic commutation rules, the transformation matrix  $T_{\mathbf{k}}$  has to satisfy a special orthonormal condition  $T_{\mathbf{k}}^\dagger \Sigma_z T_{\mathbf{k}} = \Sigma_z$ . We shall emphasize the  $\pi/2$  phase difference between  $J^+$  and  $D$ , and  $J^-$  and  $\Gamma$ , and the fact that  $J^+$  and  $D$  work in the particle or hole sector but  $J^-$  and  $\Gamma$  mix particle sector with hole sector in the magnon Hamiltonian.

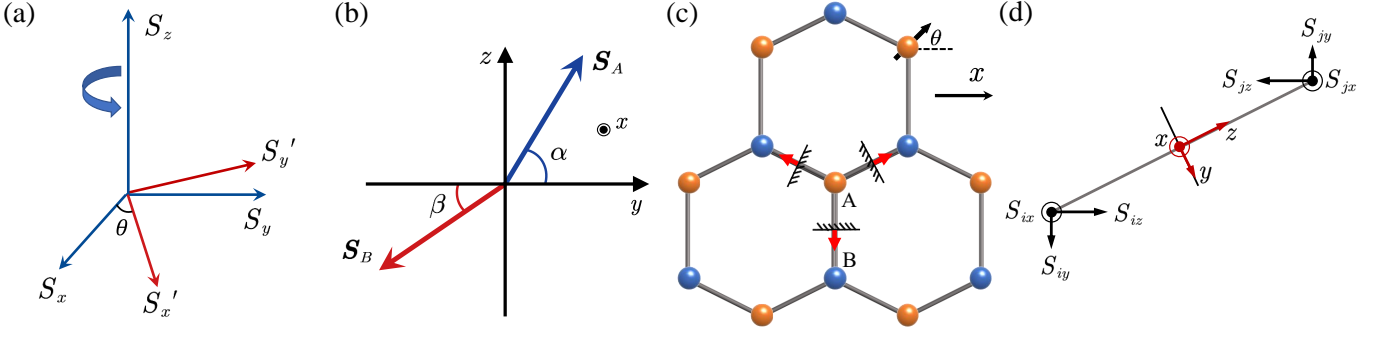

FIG. S1. (a) Rotation of local coordinate.  $S_x, S_y, S_z$  correspond to original local spin system and  $S_{x'}, S_{y'}, S_z$  represent the spin frame after rotation. (b) Spin configuration of coplanar spin-flop phase in [S8]. (c) Mirror symmetries of three nearest-neighbor bonds. Red arrows are normal vectors of mirror plane. When magnetization rotates within the plane in ferromagnetic case,  $\theta$  is the angle between magnetization and  $x$ -direction. (d) Local spin frames of site  $i$  and  $j$ . The red coordinate represents the coordinate system within the mirror plane.

## II. GAUGE FREEDOM OF CHOOSING SPIN-X DIRECTION

In this section, we will show how the rotation of the local coordinate system affects the magnon Hamiltonian and Berry curvature. At each site in a unit cell, only the spin- $z$  direction is well-defined, and any direction perpendicular to the  $z$ -th direction can equally serve as the  $x$  direction. This introduces a gauge freedom in selecting the spin- $x$  axis. However, this gauge transformation does not impact physical results, such as the Berry curvature.

Consider an initial local coordinate system with axes  $x, y$  and  $z$ , where the  $z$ -axis aligns with the orientation of the local magnetization, while  $x$  and  $y$  are chosen arbitrarily. If we rotate this coordinate system counterclockwise around  $z$ -axis by an angle  $\theta$ , we obtain a new coordinate system  $x', y', z$  as shown in Fig. S1(a).

New spin components and original ones are related by rotation matrix

$$\begin{pmatrix} S_{x'} \\ S_{y'} \end{pmatrix} = \begin{pmatrix} \cos \theta & -\sin \theta \\ \sin \theta & \cos \theta \end{pmatrix} \begin{pmatrix} S_x \\ S_y \end{pmatrix} \quad (\text{S11})$$

Thus new ladder operator  $S^{+'}$  is

$$\begin{aligned} S^{+'} &= S_{x'} + iS_{y'} \\ &= (S_x \cos \theta - S_y \sin \theta) + i(S_x \sin \theta + S_y \cos \theta) \\ &= (\cos \theta + i \sin \theta) (S_x + iS_y) \\ &= e^{i\theta} S^+ \end{aligned} \quad (\text{S12})$$

Similarly,  $S^{-'} = e^{-i\theta} S^-$ . The new ladder operators differ from the original ones by a phase factor that depends on the rotation angle. Consequently, the creation and annihilation operators are also modified by this phase factor according to Holstein-Primakoff transformation. Rotating the local coordinate of each sublattice by different angles is equivalent to applying a gauge transformation on the basis  $\psi'_{\mathbf{k}} = \mathcal{P} \psi_{\mathbf{k}}$ , where  $\mathcal{P} = \text{diag}(e^{i\theta_1}, \dots, e^{i\theta_N}, e^{-i\theta_1}, \dots, e^{-i\theta_N})$ . Then Hamiltonian will be transformed into

$$H = \sum_{\mathbf{k}} \psi_{\mathbf{k}}^\dagger \mathcal{P}^\dagger \mathcal{H}_{\mathbf{k}} \mathcal{P} \psi_{\mathbf{k}}. \quad (\text{S13})$$

As a result of this gauge transformation, the new Hamiltonian elements become  $A_{ij} e^{i(\theta_i - \theta_j)}$  and  $B_{ij} e^{i(\theta_i - \theta_j)}$ .

Due to  $\mathcal{P} \mathcal{P}^\dagger = \mathbb{I}_{2N}$  with  $\mathbb{I}_{2N}$  being  $2N \times 2N$  identity, we can demonstrate that the transformed Hamiltonian  $\mathcal{P}^\dagger \mathcal{H}_{\mathbf{k}} \mathcal{P}$  can be diagonalized by  $\mathcal{P}^\dagger T_{\mathbf{k}}$ ,

$$T_{\mathbf{k}}^\dagger \mathcal{H}_{\mathbf{k}} T_{\mathbf{k}} = (\mathcal{P}^\dagger T_{\mathbf{k}})^\dagger \mathcal{P}^\dagger \mathcal{H}_{\mathbf{k}} \mathcal{P} (\mathcal{P}^\dagger T_{\mathbf{k}}) = \begin{bmatrix} E_{\mathbf{k}} & \\ & E_{-\mathbf{k}} \end{bmatrix}. \quad (\text{S14})$$

Thus the new Berry Curvature [S7] is

$$\begin{aligned}
(\Omega_{\mu\nu})'_{n,\mathbf{k}} &= i\epsilon_{\mu\nu} \left[ \Sigma_z \frac{\partial (\mathcal{P}^\dagger T_{\mathbf{k}})^\dagger}{\partial k_\mu} \Sigma_z \frac{\partial (\mathcal{P}^\dagger T_{\mathbf{k}})}{\partial k_\nu} \right]_{nn}, \\
&= i\epsilon_{\mu\nu} \left[ \Sigma_z \frac{\partial T_{\mathbf{k}}^\dagger}{\partial k_\mu} \mathcal{P} \Sigma_z \mathcal{P}^\dagger \frac{\partial T_{\mathbf{k}}}{\partial k_\nu} \right]_{nn}, \\
&= i\epsilon_{\mu\nu} \left[ \Sigma_z \frac{\partial T_{\mathbf{k}}^\dagger}{\partial k_\mu} \Sigma_z \frac{\partial T_{\mathbf{k}}}{\partial k_\nu} \right]_{nn}, \\
&= (\Omega_{\mu\nu})_{n,\mathbf{k}},
\end{aligned} \tag{S15}$$

where we have used  $\mathcal{P}\Sigma_z\mathcal{P}^\dagger = \Sigma_z$  because they are all diagonal matrices. Thus, the Berry curvature remains unchanged under this gauge transformation, and, consequently, the thermal conductivity is also unaffected. Although additional phase factors are introduced into the Hamiltonian elements, they do not alter the physical results.

### III. EFFECTIVE TIME REVERSAL OPERATION $\mathcal{T}_x$ AND $\mathcal{T}_y$

This section discusses how effective time-reversal symmetry operates on the Hamiltonian.

The full time-reversal symmetry group  $\tilde{G}$  allows for different choices of  $C_2$  spin rotations on different sublattice sites. Besides using  $\mathcal{T}_x = TC_{2x}^s$  as effective time reversal symmetry [S9–S11] on every site, choosing  $\mathcal{T}_y = TC_{2y}^s$  as local effective time reversal symmetry on any sublattice is permitted.  $\mathcal{T}_y$  transforms creation and annihilation operators  $a_{n,i}(a_{n,i}^\dagger)$  into  $a_{n,i}(a_{n,i}^\dagger)$  rather than  $-a_{n,i}(-a_{n,i}^\dagger)$  which are transformed by  $\mathcal{T}_x$ . This can be shown by performing effective time reversal symmetry operations on ladder operators,

$$\begin{aligned}
\mathcal{T}_x S_{n,i}^\pm &= TC_{2x}^s (S_{n,i}^x \pm iS_{n,i}^y) \\
&= -(S_{n,i}^x \pm iS_{n,i}^y) \\
&= -S_{n,i}^\pm,
\end{aligned} \tag{S16}$$

while  $\mathcal{T}_y$  is different

$$\begin{aligned}
\mathcal{T}_y S_{n,i}^\pm &= TC_{2y}^s (S_{n,i}^x \pm iS_{n,i}^y) \\
&= S_{n,i}^x \pm iS_{n,i}^y \\
&= S_{n,i}^\pm.
\end{aligned} \tag{S17}$$

It is easy to observe that  $\mathcal{T}_x$  will introduce an additional minus sign to the basis function. Thus  $\mathcal{T}_x, \mathcal{T}_y$  can be identified as  $-K$  and  $K$  respectively where  $K$  is complex conjugation. Furthermore, under the operations of  $\mathcal{T}_x$  and  $\mathcal{T}_y$ , the momentum space basis  $a_{i,\mathbf{k}}$  transforms to  $-a_{i,-\mathbf{k}}$  and  $a_{i,-\mathbf{k}}$ , respectively. Now we define their operation on momentum space Hamiltonian  $\mathcal{H}_{\mathbf{k}}$

$$\begin{aligned}
\mathcal{T}_{x(y)} \mathcal{H}_{\mathbf{k}} \mathcal{T}_{x(y)}^{-1} &= \mathcal{T}_{x(y)} e^{-i\mathbf{k}\cdot\mathbf{r}} H e^{i\mathbf{k}\cdot\mathbf{r}} \mathcal{T}_{x(y)}^{-1}, \\
&= e^{i\mathbf{k}\cdot\mathbf{r}} H^* e^{-i\mathbf{k}\cdot\mathbf{r}}, \\
&= \mathcal{H}_{-\mathbf{k}}^*.
\end{aligned} \tag{S18}$$

According to Hamiltonian element in Eq.(S9), applying complex conjugation along with transformation  $\mathbf{k} \rightarrow -\mathbf{k}$  leaves momentum  $\mathbf{k}$  unchanged

$$\begin{aligned}
A_{ij}^*(-\mathbf{k}) &= \sum_{m,n} \frac{1}{2} (J_{ni,mj}^+ + iD_{ni,mj}) e^{i\mathbf{k}\cdot(\mathbf{R}_{mj}-\mathbf{R}_{ni})} - \delta_{ij} \sum_{mnl} J_{ni,ml}^{zz}, \\
B_{ij}^*(-\mathbf{k}) &= \sum_{m,n} \frac{1}{2} (J_{ni,mj}^- - i\Gamma_{ni,mj}) e^{i\mathbf{k}\cdot(\mathbf{R}_{mj}-\mathbf{R}_{ni})}.
\end{aligned} \tag{S19}$$

As a result, parameters coupled with imaginary unit  $i$  acquire a minus sign and  $\mathcal{H}_{-\mathbf{k}}^*(J_{ij}^\pm, D_{ij}, \Gamma_{ij})$  can be written as  $\mathcal{H}_{\mathbf{k}}(J_{ij}^\pm, -D_{ij}, -\Gamma_{ij})$ .

#### IV. PROOF OF ONSAGER'S RELATIONS

In this section, we aim to derive two Onsager's relations, i.e., Eq.(7) and Eq.(8) in the manuscript.

##### A. First Onsager's Relation

Firstly, we replace the original parameter sets  $(J_{ij}^\pm, D_{ij}, \Gamma_{ij})$  with new time-reversed parameter sets  $(J_{ij}^\pm, -D_{ij}, -\Gamma_{ij})$  as discussed in Sec. III. Then Berry curvature changes as follows:

$$\mathcal{T}_x[(\Omega_{\mu\nu})_{n,\mathbf{k}}(J^\pm, D, \Gamma)]\mathcal{T}_x^{-1} = (\Omega_{\mu\nu})_{n,\mathbf{k}}(J^\pm, -D, -\Gamma). \quad (\text{S20})$$

For simplicity, we omit the subscripts  $ni, mj$  here. Alternatively, we may consider the effect of  $\mathcal{T}_x$  on the wave function itself, leading to the following transformation

$$\begin{aligned} \mathcal{T}_x[(\Omega_{\mu\nu})_{n,\mathbf{k}}(J^\pm, D, \Gamma)]\mathcal{T}_x^{-1} &= i\epsilon_{\mu\nu} \left\{ \Sigma_z \frac{\partial [T_{-\mathbf{k}}^*(J^\pm, D, \Gamma)]^\dagger}{\partial k_\mu} \Sigma_z \frac{\partial T_{-\mathbf{k}}^*(J^\pm, D, \Gamma)}{\partial k_\nu} \right\}_{nn}, \\ &= i\epsilon_{\mu\nu} \left\{ \Sigma_z \frac{\partial T_{-\mathbf{k}}^T(J^\pm, D, \Gamma)}{\partial k_\mu} \Sigma_z \frac{\partial T_{-\mathbf{k}}^*(J^\pm, D, \Gamma)}{\partial k_\nu} \right\}_{nn}. \end{aligned} \quad (\text{S21})$$

Since we are only concerned with the diagonal elements, transposing the matrix does not alter the final result. Thus, we obtain

$$\begin{aligned} \mathcal{T}_x[(\Omega_{\mu\nu})_{n,\mathbf{k}}(J^\pm, D, \Gamma)]\mathcal{T}_x^{-1} &= i\epsilon_{\mu\nu} \left\{ \Sigma_z \frac{\partial T_{-\mathbf{k}}^\dagger(J^\pm, D, \Gamma)}{\partial k_\nu} \Sigma_z \frac{\partial T_{-\mathbf{k}}(J^\pm, D, \Gamma)}{\partial k_\mu} \right\}_{nn}, \\ &= -(\Omega_{\mu\nu})_{n,-\mathbf{k}}(J^\pm, D, \Gamma). \end{aligned} \quad (\text{S22})$$

These two relations lead to the following conclusion

$$(\Omega_{\mu\nu})_{n,\mathbf{k}}(J_{ij}^\pm, D_{ij}, \Gamma_{ij}) = -(\Omega_{\mu\nu})_{n,-\mathbf{k}}(J_{ij}^\pm, -D_{ij}, -\Gamma_{ij}). \quad (\text{S23})$$

Additionally, eigen equation of  $\mathcal{H}_{\mathbf{k}}$  reads

$$\Sigma_z \mathcal{H}_{\mathbf{k}}(J^\pm, D, \Gamma) T_{\mathbf{k}}(J^\pm, D, \Gamma) = T_{\mathbf{k}}(J^\pm, D, \Gamma) \begin{bmatrix} E_{\mathbf{k}}(J^\pm, D, \Gamma) & \\ & E_{-\mathbf{k}}(J^\pm, D, \Gamma) \end{bmatrix} \quad (\text{S24})$$

and eigen equation of  $\mathcal{H}_{-\mathbf{k}}^*$  is

$$\Sigma_z \mathcal{H}_{-\mathbf{k}}^*(J^\pm, D, \Gamma) T_{-\mathbf{k}}^*(J^\pm, D, \Gamma) = T_{-\mathbf{k}}^*(J^\pm, D, \Gamma) \begin{bmatrix} E_{-\mathbf{k}}(J^\pm, D, \Gamma) & \\ & E_{\mathbf{k}}(J^\pm, D, \Gamma) \end{bmatrix}. \quad (\text{S25})$$

By changing parameter set, we obtain

$$\Sigma_z \mathcal{H}_{\mathbf{k}}(J^\pm, -D, -\Gamma) T_{\mathbf{k}}(J^\pm, -D, -\Gamma) = T_{\mathbf{k}}(J^\pm, D, \Gamma) \begin{bmatrix} E_{\mathbf{k}}(J^\pm, -D, -\Gamma) & \\ & E_{-\mathbf{k}}(J^\pm, -D, -\Gamma) \end{bmatrix}. \quad (\text{S26})$$

Thus energy dispersion satisfies the relation  $\varepsilon_{n,\mathbf{k}}(J^\pm, D, \Gamma) = \varepsilon_{n,-\mathbf{k}}(J^\pm, -D, -\Gamma)$ . Combining these conclusions, we have

$$\begin{aligned} \kappa_{\mu\nu}(J^\pm, D, \Gamma) &= -\frac{k_B^2 T}{\hbar (2\pi)^2} \sum_{n=1}^N \int c_2 [\rho(\varepsilon_{n,\mathbf{k}}(J^\pm, D, \Gamma))] (\Omega_{\mu\nu})_{n,\mathbf{k}}(J^\pm, D, \Gamma) d^2k, \\ &= -\frac{k_B^2 T}{\hbar (2\pi)^2} \sum_{n=1}^N \int c_2 [\rho(\varepsilon_{n,-\mathbf{k}}(J^\pm, -D, -\Gamma))] [-(\Omega_{\mu\nu})_{n,-\mathbf{k}}(J^\pm, -D, -\Gamma)] d^2k, \\ &= -\kappa_{\mu\nu}(J^\pm, -D, -\Gamma). \end{aligned} \quad (\text{S27})$$

Therefore, the first Onsager's relation for thermal conductivity is

$$\kappa_{\mu\nu}(J_{ij}^{\pm}, -D_{ij}, -\Gamma_{ij}) = -\kappa_{\mu\nu}(J_{ij}^{\pm}, D_{ij}, \Gamma_{ij}). \quad (\text{S28})$$

When spin-orbit-locking interactions are present, particle-particle pairing terms (i.e.,  $a_i^{\dagger}a_j^{\dagger}$  or  $a_ia_j$ ) emerge in the magnon BdG Hamiltonian, causing the non-conservation of the total number of magnons. According to the analysis in Sec. I,  $J^-$  and  $\Gamma$  exhibit this effect. Under this condition, a modified thermal conductivity is given by[S7]

$$\kappa_{\mu\nu} = -\frac{k_B^2 T}{\hbar(2\pi)^2} \sum_{n=1}^N \int_{BZ} \left\{ c_2[\rho(\varepsilon_{n,\mathbf{k}})] - \frac{\pi^2}{3} \right\} (\Omega_{\mu\nu})_{n,\mathbf{k}} d^2k. \quad (\text{S29})$$

Notably, our proof remains valid despite the presence of the  $-\pi^2/3$  factor.

## B. Second Onsager's Relation

Now we choose to apply effective time-reversal symmetry in a non-uniform manner. We divide the spins within a unit cell into two groups: the time-reversal operation  $\mathcal{T}_x$  acts on spins in the first group, while  $\mathcal{T}_y$  acts on spins in the remaining group. The total effective time reversal symmetry is  $\mathcal{T} = (-KI_{n_1}) \oplus (KI_{n_2})$  where  $n_1$  and  $n_2$  are the number of spins in these two groups. Accordingly, parameters are separated into two types  $(J_{ij}^{\pm, \text{intra}}, D_{ij}^{\text{intra}}, \Gamma_{ij}^{\text{intra}})$  and  $(J_{ij}^{\pm, \text{inter}}, D_{ij}^{\text{inter}}, \Gamma_{ij}^{\text{inter}})$ . When site  $i$  and site  $j$  are in the same group, there will not be an extra minus sign after effective time reversal operation. Thus intra-group parameters change as we discussed in Sec. IV A,  $(J_{ij}^{\pm, \text{intra}}, D_{ij}^{\text{intra}}, \Gamma_{ij}^{\text{intra}}) \rightarrow (J_{ij}^{\pm, \text{intra}}, -D_{ij}^{\text{intra}}, -\Gamma_{ij}^{\text{intra}})$ . While site  $i$  and  $j$  belong to different groups, the extra minus sign multiplied with  $(\mathcal{H}_{-\mathbf{k}}^*)_{ij}$  given by  $\mathcal{T}$  can not be canceled out and new parameter set will be  $(-J_{ij}^{\pm, \text{inter}}, D_{ij}^{\text{inter}}, \Gamma_{ij}^{\text{inter}})$  due to this extra minus sign. For example,  $\mathcal{T}_{ij} = \mathcal{T}_x^i \otimes \mathcal{T}_y^j$ ,

$$\begin{aligned} \mathcal{T}_{ij} A_{ij}^{\text{inter}}(\mathbf{k}) \mathcal{T}_{ij}^{-1} &= \sum_{m,n} \frac{1}{2} \left( -J_{ni,mj}^{+, \text{inter}} - i D_{ni,mj}^{\text{inter}} \right) e^{i\mathbf{k} \cdot (\mathbf{R}_{mj} - \mathbf{R}_{ni})}, \\ \mathcal{T}_{ij} B_{ij}^{\text{inter}}(\mathbf{k}) \mathcal{T}_{ij}^{-1} &= \sum_{m,n} \frac{1}{2} \left( -J_{ni,mj}^{-, \text{inter}} + i \Gamma_{ni,mj}^{\text{inter}} \right) e^{i\mathbf{k} \cdot (\mathbf{R}_{mj} - \mathbf{R}_{ni})}. \end{aligned} \quad (\text{S30})$$

Compared with Eq.(S9),  $J_{ni,mj}^{+}$  and  $J_{ni,mj}^{-}$  are inverted. The remainder of the proof follows the same steps as in Sec. IV A, with the only difference being the modified parameter set. Consequently, the second Onsager's relation is

$$\kappa_{\mu\nu}(J_{ij}^{\pm, \text{intra}}, -D_{ij}^{\text{intra}}, -\Gamma_{ij}^{\text{intra}}, -J_{ij}^{\pm, \text{inter}}, D_{ij}^{\text{inter}}, \Gamma_{ij}^{\text{inter}}) = -\kappa_{\mu\nu}(J_{ij}^{\pm, \text{intra}}, D_{ij}^{\text{intra}}, \Gamma_{ij}^{\text{intra}}, J_{ij}^{\pm, \text{inter}}, D_{ij}^{\text{inter}}, \Gamma_{ij}^{\text{inter}}). \quad (\text{S31})$$

Alternatively, we can still use  $\mathcal{T}_x$  in the second group but rotate the local coordinates counterclockwise by  $\pi/2$  making original  $y$ -axis the new  $x$ -axis. The phase factor associated with this transform is  $e^{i\pi/2}$  which is simply imaginary unit  $i$ . This will cause a gauge transform on Hamiltonian as we discussed in Sec. II. The intra-group parameters remain the same because they share the same coordinate, causing the phase factor to cancel out. However, for the inter-group parameters, an additional factor of  $i$  appears, so that  $J_{ij}^{\pm}$  is now coupled with  $i$ , instead of  $D_{ij}$  and  $\Gamma_{ij}$ , e.g.  $(J_{ij}^{+} + i D_{ij}) \rightarrow (i J_{ij}^{+} - D_{ij})$ . Under effective times reversal symmetry  $\mathcal{T}_x$  as discussed in Sec. IV A, new parameter set will be  $(-J_{ij}^{\pm}, D_{ij}, \Gamma_{ij})$ . This analysis is consistent with Eq.(S31).

## V. DETAILS OF HONEYCOMB LATTICE MODELS

The content of this section contains details of two honeycomb lattice models with in-plane magnetization in the main text.

### A. Antiferromagnetic order

In honeycomb lattice with in-plane antiferromagnetic order, the nearest-neighbor interaction tensor  $\mathcal{J}_{ij}$  is given by

$$\mathcal{J}_{ij} = \begin{pmatrix} -J^{+} - J^{-} & w_{ij}\Gamma & 0 \\ w_{ij}\Gamma & -J^{+} + J^{-} & 0 \\ 0 & 0 & -J_0 \end{pmatrix} \quad (\text{S32})$$

where  $J^+$  and  $J_0$  are isotropic exchange interaction from Heisenberg interaction,  $J^-$  and  $\Gamma$  are diagonal and off-diagonal part of symmetric anisotropic interaction. Due to the mirror planes perpendicular to the nearest-neighbor bonds are retained in the manuscript, only components of spin fluctuations lying within the mirror plane contribute to the Hamiltonian. The three nearest-neighbor vectors  $\mathbf{a}_i$  are  $\mathbf{a}_1 = (\sqrt{3}/2, 1/2)$ ,  $\mathbf{a}_2 = (0, -1)$  and  $\mathbf{a}_3 = (-\sqrt{3}/2, 1/2)$ . When considering  $\mathbf{a}_1$  as shown in FIG. S1(d), spin-x axis aligns with the  $x$  axis in mirror plane, only spin-y is needed to be decomposed, i.e.,  $S_{iy} \rightarrow \sqrt{3}/2 S_{iy}$ ,  $S_{jy} \rightarrow -\sqrt{3}/2 S_{jy}$ . This is equivalent to decomposing the equilibrium direction of magnetization along the normal direction of the mirror plane as illustrated by red arrows in FIG. S1(c). In other words, direction of magnetization on site  $i$  is  $(1, 0)$  and the normal vector is  $(\sqrt{3}/2, 1/2)$ , leading to  $w_{ij} = \sqrt{3}/2$ . Finally, the matrix element of antiferromagnetic honeycomb lattice is given by

$$\mathcal{H}_{\mathbf{k}} = \frac{S}{2} \begin{bmatrix} 3J_0 + B & J^- f(\mathbf{k}) + i\Gamma l(\mathbf{k}) & 0 & -J^+ f(\mathbf{k}) \\ J^- f^*(\mathbf{k}) - i\Gamma l^*(\mathbf{k}) & 3J_0 - B & -J^+ f^*(\mathbf{k}) & 0 \\ 0 & -J^+ f(\mathbf{k}) & 3J_0 + B & J^- f(\mathbf{k}) - i\Gamma l(\mathbf{k}) \\ -J^+ f^*(\mathbf{k}) & 0 & J^- f^*(\mathbf{k}) + i\Gamma l^*(\mathbf{k}) & 3J_0 - B \end{bmatrix}. \quad (\text{S33})$$

where  $f(\mathbf{k}) = \sum_i \exp(i\mathbf{k} \cdot \mathbf{a}_i)$ ,  $l(\mathbf{k}) = \sum_i w_{0i} \exp(i\mathbf{k} \cdot \mathbf{a}_i)$ . In FIG.2(b) of the manuscript,  $J^-$  and  $\Gamma$  are parameterized as  $J^- = -0.13J_0 \cos \alpha$ ,  $\Gamma = -0.13J_0 \sin \alpha$ . Besides, we set  $J^+ = \pm 0.67J_0$  which changes sign as  $\Gamma$  varies,  $B = -0.53J_0$  and  $S$  is set to 1. Finally, the Brillouin zone is divided into a  $1000 \times 1000$  grid to complete the integration.

Here, magnetic field plays the role of opening the gap and inducing nonzero Berry curvature. It is worth mentioning that in this case thermal conductivity is also an odd function of magnetic field  $\mathbf{B}$  and this is not because it breaks the effective time-reversal symmetry. Since the chiral symmetry ( $\sigma_x K$ ) reverses the sign of the magnetic field in Eq. (S33), the Berry curvature of the Hamiltonian transforms as  $\Omega_{n,\mathbf{k}}(-B)$ . Moreover, under complex conjugation, the Berry curvature flips sign, i.e.,  $\Omega_{n,\mathbf{k}}(B) \rightarrow -\Omega_{n,\mathbf{k}}(B)$ . Since these two transformations are related by the chiral symmetry operation, it follows that  $\Omega_{n,\mathbf{k}}(-B) = -\Omega_{n,\mathbf{k}}(B)$ , implying that the Berry curvature is an odd function of  $B$ . On the other hand, energy dispersion remains unchanged. Because the thermal Hall conductivity  $\kappa_{xy}$  is determined by the integral of the Berry curvature over the Brillouin zone, it inherits this property and is an odd function of magnetic field.

## B. Ferromagnetic order

In the honeycomb lattice with in-plane ferromagnetic order, the interaction tensor remains the same as that in Sec. V A, except that the nearest-neighbor Heisenberg interaction changes sign due to the change in magnetic order. An additional staggered isotropic exchange term between second nearest neighbors has to be added to break the chiral symmetry. Thus the Hamiltonian is given by

$$H = \sum_{\langle i,j \rangle} \mathbf{S}_i^T \mathcal{J}_{ij} \mathbf{S}_j - \sum_{\langle\langle i,j \rangle\rangle} \sum_{\mu=A,B} J_\mu \mathbf{S}_i^\mu \cdot \mathbf{S}_j^\mu - \sum_i \mathbf{B} \cdot \mathbf{S}_i. \quad (\text{S34})$$

When  $J_A \neq J_B$ , the breaking of chiral symmetry leads to the opening of a band gap, which in turn induces a finite Berry curvature. Different with antiferromagnetic case, the magnetic field in this ferromagnetic model is used to rotate the equilibrium orientation of the magnetic order within the plane without affecting other parameters.

Since we now allow the magnetic order to rotate within the plane with the magnetic field, we need the angle  $\theta$  to represent the direction of magnetization as shown in FIG. S1(c). Thus the direction of magnetization is expressed as  $\mathbf{m} = (\cos \theta, \sin \theta)$ . Following the analysis in Sec. V A, the  $w_{ij}$  in ferromagnetic case are  $w_{01} = \frac{\sqrt{3}}{2} \cos \theta + \frac{1}{2} \sin \theta$ ,  $w_{02} = -\sin \theta$  and  $w_{03} = -\frac{\sqrt{3}}{2} \cos \theta + \frac{1}{2} \sin \theta$ . By combining the information in the main text, we can derive the matrix form of the momentum space Hamiltonian

$$\mathcal{H}_{\mathbf{k}} = \frac{S}{2} \begin{bmatrix} \mathcal{J}_A - J_A g(\mathbf{k}) + B & -J^+ f(\mathbf{k}) & 0 & J^- f(\mathbf{k}) + i\Gamma l(\mathbf{k}) \\ -J^+ f^*(\mathbf{k}) & \mathcal{J}_B - J_B g(\mathbf{k}) + B & J^- f^*(\mathbf{k}) + i\Gamma l^*(\mathbf{k}) & 0 \\ 0 & J^- f(\mathbf{k}) - i\Gamma l(\mathbf{k}) & \mathcal{J}_A - J_A g(\mathbf{k}) + B & -J^+ f(\mathbf{k}) \\ J^- f^*(\mathbf{k}) - i\Gamma l^*(\mathbf{k}) & 0 & -J^+ f^*(\mathbf{k}) & \mathcal{J}_B - J_B g(\mathbf{k}) + B \end{bmatrix} \quad (\text{S35})$$

where  $\mathcal{J}_{A(B)} = 3J_0 + 6J_{A(B)}$ ,  $g(\mathbf{k}) = \sum_i \cos(\mathbf{k} \cdot \mathbf{d}_i)$ ,  $f(\mathbf{k}) = \sum_i \exp(i\mathbf{k} \cdot \mathbf{a}_i)$ ,  $l(\mathbf{k}) = \sum_i w_{0i} \exp(i\mathbf{k} \cdot \mathbf{a}_i)$  with  $\mathbf{d}_i$  linking next nearest neighbors and  $\mathbf{S}_i = S\mathbf{m} = S(\cos \theta, \sin \theta)$  being magnetization in ground state. In FIG.2(d) of the manuscript, we set  $J^+ = J_0$ ,  $J^- = \Gamma = 0.2J_0$ ,  $J_A = 0.1J_0$ ,  $J_B = 0.12J_0$ ,  $B = 0.8J_0$  and  $S = 1$ . We must mention that although  $J^-$  and  $\Gamma$  are present, Chern numbers of these two systems are zero so that thermal conductivity in Eq. (S29) is equivalent to that in the manuscript.

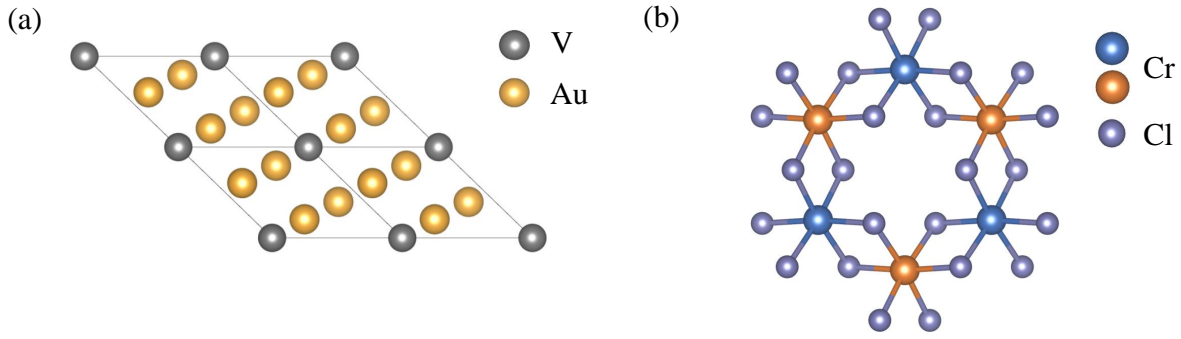

FIG. S2. Atom structures of VAu<sub>4</sub> and CrCl<sub>3</sub>. This figure is plotted by VESTA [S12]. Crystal parameters are from Material Project [S13, S14].

## VI. SYMMETRY ANALYSIS OF VAu<sub>4</sub>, CrCl<sub>3</sub> AND V<sub>2</sub>Se<sub>2</sub>O

In this section, we analyze the symmetries of VAu<sub>4</sub>, CrCl<sub>3</sub> and V<sub>2</sub>Se<sub>2</sub>O to demonstrate that these materials can host a magnon thermal Hall effect induced by symmetric anisotropic interactions.

The point group of VAu<sub>4</sub> is  $4/m$ , which includes an inversion operation. The crystal structure is illustrated in FIG. S2(a). We need to determine whether the midpoint of the V atoms is the inversion center. In the primitive crystallographic setting, the lattice parameters are  $a = b = c = 5.042\text{\AA}$ ,  $\alpha = \beta = 99.346^\circ$ , and  $\gamma = 132.469^\circ$  [S13, S14]. In fractional coordinates, we place two V atoms at  $(0,0,0)$  and  $(1,0,0)$ . Thus, the midpoint is  $\mathbf{O} = (0.5, 0, 0)$ . The positions of the Au atoms are  $(0.2051, 0.6034, 0.8085)$ ,  $(0.3966, 0.2051, 0.6016)$ ,  $(0.6034, 0.7949, 0.3984)$ , and  $(0.7949, 0.3966, 0.1915)$  [S13, S14]. The corresponding point  $\mathbf{r}_i$  after the inversion of  $\mathbf{r}_j$  should satisfy the relation  $\mathbf{r}_i = 2\mathbf{O} - \mathbf{r}_j$ . For instance, the corresponding point of  $(0.2051, 0.6034, 0.8085)$  is  $(0.7049, -0.6034, -0.8085)$ , which, after applying a spatial translation, becomes  $(0.7049, 0.3966, 0.1915)$ . The same applies to the other three Au atoms and V atoms. Hence, the middle point of V atoms is indeed an inversion center. Moreover, group  $4/m$  only contains horizontal mirror symmetry  $\sigma_h$ , thus anisotropic coupling is allowed.

Now let us turn the focus to monolayer CrCl<sub>3</sub> shown in FIG. S2(b) which possesses crystal structures of monolayer CrX<sub>3</sub> (X = Cl, I, Br). The space group for monolayer CrCl<sub>3</sub> is P-31m [S15–S17] which corresponds to point group  $D_{3d}$ . The midpoint between two Cr ions is inversion center, leading to a vanishing nearest-neighbor DM interaction [S18]. Since the two Cl ions near the nearest-neighbor bond are positioned above and below the Cr plane, only a mirror plane perpendicular to both the Cr plane and the nearest-neighbor bond exists. As a result, there is only nearest-neighbor symmetric anisotropic interaction. Moreover, what makes CrCl<sub>3</sub> more promising is the experimental observation of its in-plane easy axis [S19].

Same analysis can be carried to V<sub>2</sub>Se<sub>2</sub>O [S20]. The inversion symmetry between nearest-neighbor magnetic V atoms is retained, leading to zero DM interaction. While there is only one mirror plane which allows nonzero symmetric anisotropic interaction. Here, we must point out that in order to break chiral symmetry, a layered structure of CrCl<sub>3</sub> or V<sub>2</sub>Se<sub>2</sub>O with in-plane electric field or strain gradient is required.

- 
- [S1] T. Holstein and H. Primakoff, Field Dependence of the Intrinsic Domain Magnetization of a Ferromagnet, *Phys. Rev.* **58**, 1098 (1940).
  - [S2] A. Corticelli, R. Moessner, and P. A. McClarty, Spin-space groups and magnon band topology, *Phys. Rev. B* **105**, 064430 (2022).
  - [S3] J. Colpa, Diagonalization of the quadratic boson Hamiltonian, *Physica A: Statistical Mechanics and its Applications* **93**, 327 (1978).
  - [S4] S. Toth and B. Lake, Linear spin wave theory for single-Q incommensurate magnetic structures, *Journal of Physics: Condensed Matter* **27**, 166002 (2015).
  - [S5] R. Shindou, R. Matsumoto, S. Murakami, and J.-i. Ohe, Topological chiral magnonic edge mode in a magnonic crystal, *Phys. Rev. B* **87**, 174427 (2013).
  - [S6] A. Okamoto and S. Murakami, Berry curvature for magnons in ferromagnetic films with dipole-exchange interactions, *Phys. Rev. B* **96**, 174437 (2017).
  - [S7] R. Matsumoto, R. Shindou, and S. Murakami, Thermal Hall effect of magnons in magnets with dipolar interaction, *Phys. Rev. B* **89**, 054420 (2014).

- [S8] R. R. Neumann, A. Mook, J. Henk, and I. Mertig, Thermal Hall Effect of Magnons in Collinear Antiferromagnetic Insulators: Signatures of Magnetic and Topological Phase Transitions, [Phys. Rev. Lett. \*\*128\*\*, 117201 \(2022\)](#).
- [S9] H. Chen, Q. Niu, and A. H. MacDonald, Anomalous Hall Effect Arising from Noncollinear Antiferromagnetism, [Phys. Rev. Lett. \*\*112\*\*, 017205 \(2014\)](#).
- [S10] M.-T. Suzuki, T. Koretsune, M. Ochi, and R. Arita, Cluster multipole theory for anomalous Hall effect in antiferromagnets, [Phys. Rev. B \*\*95\*\*, 094406 \(2017\)](#).
- [S11] A. Mook, J. Henk, and I. Mertig, Thermal Hall effect in noncollinear coplanar insulating antiferromagnets, [Phys. Rev. B \*\*99\*\*, 014427 \(2019\)](#).
- [S12] K. Momma and F. Izumi, *VESTA3* for three-dimensional visualization of crystal, volumetric and morphology data, [Journal of Applied Crystallography \*\*44\*\*, 1272 \(2011\)](#).
- [S13] W. Koester and H. Nordskog, Das Zweistoffsystem Gold-Vanadium, *Zeitschrift fuer Metallkunde* **51**, 501 (1960).
- [S14] A. Jain, S. P. Ong, G. Hautier, W. Chen, W. D. Richards, S. Dacek, S. Cholia, D. Gunter, D. Skinner, G. Ceder, and K. a. Persson, Commentary: The Materials Project: A materials genome approach to accelerating materials innovation, [APL Materials \*\*1\*\*, 011002 \(2013\)](#).
- [S15] D. Mastrippolito, J. Wang, G. Profeta, and L. Ottaviano, Unconventional ferrimagnetism and enhanced magnetic ordering temperature in monolayer CrCl<sub>3</sub> by introducing O impurities and Cl vacancies, [Journal of Physics: Materials \*\*5\*\*, 014004 \(2022\)](#).
- [S16] Y. Gao, J. Wang, Y. Li, M. Xia, Z. Li, and F. Gao, Point-Defect-Induced Half Metal in CrCl<sub>3</sub> Monolayer, [physica status solidi \(RRL\) – Rapid Research Letters \*\*12\*\*, 1800105 \(2018\)](#).
- [S17] S.-D. Guo, [External-field-induced altermagnetism in experimentally synthesized monolayer CrX<sub>3</sub> \(x=cl, br and i\) \(2025\)](#), [arXiv:2503.23036 \[cond-mat.mtrl-sci\]](#).
- [S18] D. Šabani, C. Bacaksiz, and M. V. Milošević, Ab initio methodology for magnetic exchange parameters: Generic four-state energy mapping onto a Heisenberg spin Hamiltonian, [Phys. Rev. B \*\*102\*\*, 014457 \(2020\)](#).
- [S19] A. Bedoya-Pinto, J.-R. Ji, A. K. Pandeya, P. Gargiani, M. Valvidares, P. Sessi, J. M. Taylor, F. Radu, K. Chang, and S. S. P. Parkin, Intrinsic 2D-XY ferromagnetism in a van der Waals monolayer, [Science \*\*374\*\*, 616 \(2021\)](#).
- [S20] H.-Y. Ma, M. Hu, N. Li, J. Liu, W. Yao, J.-F. Jia, and J. Liu, Multifunctional antiferromagnetic materials with giant piezomagnetism and noncollinear spin current, [Nature Communications \*\*12\*\*, 2846 \(2021\)](#).
